# Supplementary material for: Mechanics-Aware Modeling of Cloth Appearance
Source: arXiv:1904.11116 source file (2019-10-10)
Supplement: Supplementary file 1 [file appendix.tex]

\section{Details of Parameter Homogenization}\label{sec:param_fit}
Here we present the details of our parameter fitting process discussed in \secref{param}.
First, we define the energy function for external force,
$\psi(\bm{R}) = g(\bm{R}_2) + h(\bm{R}_3)$. Again, we note that here, unlike~\cite{jiang2017anisotropic}, 
we neglect the elastic stretching energy, because it is already considered in the elastic rod model together with the 
bending and twisting energies, which the work of~\cite{jiang2017anisotropic} ignores.

Now, consider a yarn at static equilibrium in fiber-level simulation. Its
centerline indicates the expected static equilibrium state of the same yarn
under the same external load in yarn-level simulation (when the material
parameters are properly set).  In this case, the yarn's external forces are
balanced against the internal forces, which, as described in \secref{param},
can be estimated using the elastic rod model applying to the centerline. We
denote the external force estimated in this way as $\bm{f}_{v}(\bm{x})$, 
which is defined on each yarn vertex $v$ located at $\bm{x}$ (recall \figref{polyline}).

In the Lagrangian/Eulerian approach~\cite{jiang2017anisotropic,fei2018mms}, the simulation also exploits a background
Eulerian grid. Forces on yarn vertices are transferred to the grid using kernel interpolation,
\begin{equation}\label{eq:fext0}
\tilde{\bm{f}}^*_{i} = \sum_{v} w_{iv}(\bm{x})\bm{f}_v(\bm{x}),
\end{equation}
where $\tilde{\bm{f}}_{i}$ is the estimated external force at a grid node $i$, and $w_{iv}(\bm{x})$ is the kernel 
function for interpolating the force from yarn vertex $v$ to grid node $i$.
On the other hand, the external force on the grid can be expressed by taking the derivative of $\psi(\bm{R})$
with respect to vertex positions of the yarn and then transferring the force to the grid. 
The expression, derived in~\cite{jiang2017anisotropic}, is 
\begin{equation}\label{eq:fext1}
\tilde{\bm{f}}_{i} = -\sum_{v}\sum_{\beta=2}^{3} V_v^0 \frac{\partial \psi}{\partial \bm{F}_\beta} \bm{d}^T_\beta\nabla w_{iv}(\bm{x}),
\end{equation}
where the scalar $V_v^0$ is the effective volume of vertex $v$, $\bm{d}_\beta$ is the $\beta^\textrm{th}$ column 
of the matrix $\bm{d}=\bm{F}\bm{D}$. Here recall that $\bm{F}$ is the deformation gradient and $\bm{D}$ (introduced in \secref{param}) 
is the $3\times3$ matrix indicating local material directions. Both are defined on the finite elements of the polylines.
Equating~\eq{fext1} with~\eq{fext0} results in a system of linear equations with respect to $\frac{\partial\psi}{\partial\bm{F}_\beta}$.
Here, the number of equations is a triple of the grid size, and the number of unknowns is six times of the total number of yarn vertices 
(because $\frac{\partial\psi}{\partial\bm{F}_2}$ and $\frac{\partial\psi}{\partial\bm{F}_3}$ have six elements).
In practice, this is an over-constrained linear system, and $\frac{\partial\psi}{\partial\bm{F}_\beta}$ can be obtained uniquely
through a least-squares solve.

Next, we consider each edge $\bm{e}$ on yarn polylines. From the relationship $\bm{d}=\bm{F}\bm{D}$, we notice that
$\frac{\partial\psi}{\partial\bm{d}}=\frac{\partial\psi}{\partial\bm{F}}\bm{D}^{-T}$ and
\begin{equation}\label{eq:ff2}
\frac{\partial\psi}{\partial\bm{d}} = 
\bm{Q}\left( \mathsf{T}[\bm{K}] + \mathsf{T}[\bm{K}]^T - \mathsf{D}[\bm{K}]\right)\bm{R}^{-T}.
\end{equation}
The latter is derived in~\cite{jiang2017anisotropicb}, in which $\mathsf{T}[\cdot]$
and $\mathsf{D}[\cdot]$ are matrix operators that return the upper triangular and diagonal parts of the matrix, respectively,
and $\bm{Q}$ and $\bm{R}$ are results from the QR-decomposition of $\bm{F}\bm{D}$, as introduced in \secref{param},
and $\bm{K}=\frac{\partial\psi}{\partial\bm{R}}\bm{R}^T$.

At this point, we have obtained $\frac{\partial\psi}{\partial\bm{F}}$ from the above least-squares solve.
Using Eq.~\eq{ff2}, we compute the upper triangular part of $\bm{K}$ by
\begin{equation}
\tilde{\bm{K}} = \bm{Q}^T \frac{\partial\psi}{\partial\bm{F}}\bm{D}^{-T} \bm{R}^T.
\end{equation}
In the resulting $\tilde{\bm{K}}$, only its upper triangular part is same as $\bm{K}$ (i.e., $\mathsf{T}[\tilde{\bm{K}}] = \mathsf{T}[\bm{K}]$).
Fortunately, we observe the following relationships, 
\begin{equation}
\mathsf{T}[\tilde{\bm{K}}\bm{R}^{-T}] = \mathsf{T}[\bm{K}\bm{R}^{-T}] = \mathsf{T}[\frac{\partial\psi}{\partial\bm{R}}],
\end{equation}
which can be easily verified by noticing that $\bm{R}$ is an upper triangular matrix.
Furthermore, because $\frac{\partial\psi}{\partial\bm{R}}$ is also an upper triangular matrix, we can compute this matrix
by evaluating $\tilde{\bm{K}}\bm{R}^{-T}$ and ignoring its lower triangular part.

Finally, we express $\frac{\partial\psi}{\partial\bm{R}}$ analytically. Since
$\psi(\bm{R})=g(\bm{R}_2)+h(\bm{R}_3)$ is a quadratic form, its derivative with
respect to $\bm{R}$ is a linear function with respect to its coefficients,
$a_i$ and $b_i$ ($i=1,2,3$). We denote this linear function using $L_{\bm{R}}(a_i,b_i)$. This leads
to a system of linear equations,
$$
L_{\bm{R}}(a_1,a_2,a_3,b_1,b_2,b_3) = \frac{\partial\psi}{\partial\bm{R}},
$$
where the value on the right-hand side is computed from the previous step. Each of the equations corresponds to 
a $\frac{\partial\psi}{\partial\bm{R}}$ value evaluated at an edge $\bm{e}$. When solving this system in a least-squares fashion, we must 
also ensure that $g(\bm{R}_2)$ and $h(\bm{R}_3)$ are both positive semidefinite, or the matrices,
$$
\bm{A} = \begin{bmatrix}
a_1 & \frac{1}{2}a_2 \\
\frac{1}{2}a_2 & a_3
\end{bmatrix}
\;\textrm{and}\;
\bm{B} = \begin{bmatrix}
b_1 & \frac{1}{2}b_2 \\
\frac{1}{2}b_2 & b_3
\end{bmatrix},
$$
must be positive semidefinite. This imposes a conic constraint, and the problem is a classic
semidefinite-quadratic-linear programming problem, which we solve using the SDPT3 solver~\cite{tutuncu2003solving}.

% force balance
% force formula

% simulated state
%% In practice, we reuse the fiber-level simulation results generated for
